# Supplementary material for: Learning to Teach Fairness-aware Deep Multi-task Learning
Source: arXiv:2206.08403 source file (2022-06-16)
Supplement: Supplementary file 1 [file appendix.tex]

%\appendix
\section*{Appendix}
\subsection*{Important Notations}
Important notations are summarised in Table~\ref{tab:notation}.
\begin{table}[httb!]
\caption{Important notations and corresponding descriptions.}\label{tab:notation}
\begin{tabular}{@{}ll@{}}
\hline
\textbf{Notations}             & \textbf{Descriptions} \\ \hline
\multicolumn{1}{l|}{t, T }& task index, total number of tasks  \\
\multicolumn{1}{l|}{S, $g$, $\overline{g}$}  & binary protected attribute, protected group, non-protected group      \\
%\multicolumn{1}{l|}{$g$ ($\overline{g}$)}  &  protected (non-protected) groups based on $S$\\
%that historically faced discrimination
\multicolumn{1}{l|}{$U$}  & non-protected attributes \\
\multicolumn{1}{l|}{$\mathcal{L}_t()$}  & accuracy loss in task $t$ \\
\multicolumn{1}{l|}{$\mathcal{F}_t()$} &  fairness loss in task $t$ \\
\multicolumn{1}{l|}{$\mathcal{M}$ (Q)}  & Deep MTL network (resp. DQN network) \\
\multicolumn{1}{l|}{$\theta (\theta^Q)$} & learning parameter space of $\mathcal{M}$ (resp. $Q$)  \\
\multicolumn{1}{l|}{$\theta_t (\theta_t^Q$)} & parameters of the task-specific layers of $\mathcal{M}$ (resp. $Q$) \\
\multicolumn{1}{l|}{$\theta_{sh} (\theta_{sh}^Q)$} & parameters of the shared layers of $\mathcal{M}$ (resp. $Q$) \\
\multicolumn{1}{l|}{$w_t,\omega_t$} &  weight to quantify gradient update for task t of M and Q \\
\multicolumn{1}{l|}{$\nabla_{\theta_t},\nabla_{\theta_{sh}}$} & gradient w.r.t $\theta_t$, $\theta_{sh}$\\
\multicolumn{1}{l|}{$L_{grad}$} & Loss function used to learn $w_t,\omega_t$\\
\hline
\end{tabular}
\end{table}
\subsection*{Detailed info of Data}\label{appendix:data}
\noindent \textbf{Tabular data: ACS-PUMS} 
We use the recently released  American Community Survey Public Use Microdata Sample data which comprises a reconstruction of the famous Adult dataset~\cite{ding2021retiring}. We formulate the MTL problem by picking 5 different well defined binary classification tasks from their repository\footnote{\url{https://github.com/zykls/folktables}}, the individual tasks are provided in Table~\ref{tab:datasets}.
We use \textit{gender} as the protected attribute with \textit{female} as the protected group. 
For training we use the census data across all states from the year ``2018", divided into train (70\%) and validation (30\%) sets. For testing we use the data from the following year ``2019" (both years of size $\approx 1.65M$). 

\noindent\textbf{Visual data: CelebA-Gender} We use the CelebA dataset~\cite{liu2015celebA} consisting of $202.5K$ celebrity facial images and 40 different binary attributes. We use the provided\footnote{\url{http://mmlab.ie.cuhk.edu.hk/projects/CelebA.html}} partitioning into train (\#162,770 instances), validation (\#19,867 instances), and test (\#19,962 instances) set. 
%All attributes are binary and a prediction task for each attribute can be availed from this dataset.
\emph{Gender} is treated as the protected attribute with \textit{female} as the protected group. 
There are attributes that are true mainly in the protected or non-protected groups. For example, the attribute ``Mustache'' is true mainly for the male group (only 3 female instanceshave positive labels). We filter out such attributes from the MTL formulation. Namely, we consider only attributes which have a minimum number of true values for either protected or non-protected groups (we set the threshold to 2.5K instances or 1.5\%). After filtering, we are left with 17 different binary attributes which comprise the different tasks for the MTL and are presented in Table~\ref{tab:datasets}.

\noindent\textbf{Visual data: CelebA-Age} We use again the CelebA dataset with the provided train, validation, and test partitions as before, but this time we use \textit{Age} as the protected attribute with \textit{old} being the protected group. Applying the above filtering, we are left with $31$ binary attributes which comprise the different MTL tasks and are presented in Table~\ref{tab:datasets}. 
\begin{table}
\caption{Overview of datasets (the protected value is underlined)}
    \label{tab:datasets}
    \centering
    \begin{tabular}{p{0.10\linewidth}|p{0.15\linewidth}|p{0.15\linewidth}|p{0.1\linewidth}|p{0.5\linewidth}}\hline
    \textbf{Dataset} & \textbf{Type} &  \textbf{Protected attribute } & \textbf{\#tasks} & \textbf{MTL tasks} \\\hline
    \textbf{ACS-PUMS} & Tabular & Gender: \{\textit{male}, \textit{\underline{female}}\} & 5 &  \textit{Employment status}, \textit{Income prediction}, \textit{Health Insurance status}, \textit{Work Travel time}, \textit{Income-poverty ratio status}\\\hline
    \textbf{CelebA-Gender} & Image  &Gender: \{\textit{male}, \textit{\underline{female}}\} & 17 &  \textit{Attractive}, \textit{Bags Under Eyes}, \textit{Bangs}, \textit{Big Lips}, \textit{Big Nose}, \textit{Black Hair}, \textit{Brown Hair} , \textit{Bushy Eyebrows}, \textit{High Cheekbones}, \textit{Mouth Slightly Open}, \textit{Narrow Eyes}, \textit{Oval Face}, \textit{Pointy Nose}, \textit{Smiling}, \textit{Straight Hair}, \textit{Wavy Hair}, \textit{Age}\\\hline
    \textbf{CelebA-Age} & Image &Age: \{\textit{young}, \textit{\underline{old}}\} &31 &  \textit{5 o'clock Shadow}, \textit{Arched Eyebrows}, \textit{Attractive}, \textit{Bags Under Eyes}, 
 \textit{Bangs}, \textit{Big Lips}, \textit{Big Nose}, \textit{Black Hair}, \textit{Blond Hair}, \textit{Brown Hair} , \textit{Bushy Eyebrows}, 
 \textit{Eyeglasses}, \textit{Goatee}, \textit{Heavy Makeup}, \textit{High Cheekbones}, 
 \textit{Gender}, \textit{Mouth Slightly Open}, \textit{Mustache}, \textit{Narrow Eyes},  \textit{No Beard}, \textit{Oval Face}, \textit{Pointy Nose}, \textit{Receding Hairline}, 
 \textit{Sideburns}, \textit{Smiling}, \textit{Straight Hair}, \textit{Wavy Hair}, 
 \textit{Wearing Earrings}, \textit{Wearing Lipstick}, \textit{Wearing Necklace}, 
 \textit{Wearing Necktie}\\\hline
    \end{tabular}
    
\end{table}

\subsection*{Setup and parameter tuning}\label{sec:repro}
We run all our experiments using Pytorch 1.7.1\footnote{https://pytorch.org/} framework, with training batch size of 8,192 instances. %To shuffle the data we use pytorch random permute with seed 0. 
For train, validation split wherever required, we use sklearn\footnote{https://scikit-learn.org/stable/} with random seed 9. 
For the visual data (CelebA-Gender, CelebA-Age), like~\cite{MTLfairWang0BPCC21}, we use ResNet-18\footnote{https://pytorch.org/vision/stable/models.html} without the final layer and without fine tuning to generate feature representation. 
For optimising the models we use the AdamW\footnote{https://pytorch.org/docs/stable/generated/torch.optim.AdamW.html} optimizer. 
For each method, the same network architecture is used. For the shared parameters we use 4 fully connected layers consisting of 1,024, 1,024, 512, 128 neurons with ReLU activation respectively. For the task specific parameters we use a single fully connected layer of 2 neurons with soft-max activation for each task. 
The \verb|STL| model for computing  $ARA$ and $AREO$ scores is a neural network with parameters and architecture as of an \verb|MTL| with $T=1$ i.e., in place of $T$ task specific layers we have only a single fully connected layer of 2 neurons, trained only on task $t$ with the objective loss function as in Eq~\ref{eq:fair_stl}. 
For the \emph{MTA-F} method, we tune the accuracy-fairness trade-off weights $\lambda_t$ following the original paper~\cite{MTLfairWang0BPCC21}.  
The link to our code is given here\footnote{https://anonymous.4open.science/r/L2TFMT-F309/}.
